# Supplementary material for: Moduli Space of SU(2) Singular Monopole
Source: arXiv:2507.13424 source file (2025-07-17)
Supplement: Supplementary file 1 [file AppendixB.tex]

% Appendix B

\chapter{Useful }
\begin{eqnarray}
\partial_i r^2 &=& 2r_i\nonumber\\
\partial_i r &=& \frac{r_i}{r}\nonumber\\
\partial_i z &=& \frac{z_i}{z}\nonumber\\
\partial_i (z+d)^2 &=& 2\frac{z_i}{z}(z+d)\nonumber\\
\partial_i \sinh 2\lambda r &=& \frac{2\lambda r_i}{r}\cosh 2\lambda r\nonumber\\
\partial_i \cosh 2\lambda r &=& \frac{2\lambda r_i}{r}\sinh 2\lambda r\nonumber\\
\partial_i \mathcal{L} &=& \left(2\frac{z_i}{z}(z+d)+2r_i\right)\sinh 2\lambda r+\left((z+d)^2+r^2\right)\left(\frac{2\lambda r_i}{r}\cosh 2\lambda r\right)\nonumber\\
&& +2\frac{r_i}{r}(z+d)\cosh 2\lambda r+2r\frac{z_i}{z}\cosh 2\lambda r+2r (z+d)\frac{2\lambda r_i}{r}\sinh 2\lambda r\nonumber\\
\partial_i \mathcal{L}^{-1} &=& -\frac{\partial_i \mathcal{L}}{\mathcal{L}^2}\nonumber\\
\partial_i \sinh^2 \lambda r&=&\frac{2\lambda r_i}{r}\cosh 2\lambda r\sinh 2\lambda r\nonumber \\
\partial_i \mathcal{D}&=&2\frac{z_i}{z}(z+d)-2r_i\nonumber\\
\partial_i \frac{1}{r^2} &=& -\frac{2 r_i}{r^4}\nonumber\\
\partial_i \coth 2\lambda r &=& -\frac{2\lambda r_i}{r} \mathrm{cosech}^2 2\lambda r
\end{eqnarray}
